# Supplementary material for: Association between productivity and journal impact across disciplines and career age
Source: arXiv:2108.02920 source file (2021-08-06)
Supplement: Supplementary file 1 [file prr_supplementary.pdf]

# Association between productivity and journal impact across disciplines and career age

Andre S. Sunahara,[1] Matjaž Perc,[2,3,4,5] and Haroldo V. Ribeiro[1,*]

[1] *Departamento de Física, Universidade Estadual de Maringá – Maringá, PR 87020-900, Brazil*
[2] *Faculty of Natural Sciences and Mathematics, University of Maribor, Koroška cesta 160, 2000 Maribor, Slovenia*
[3] *Department of Medical Research, China Medical University Hospital, China Medical University, Taichung, Taiwan*
[4] *Alma Mater Europaea ECM, Slovenska ulica 17, 2000 Maribor, Slovenia*
[5] *Complexity Science Hub Vienna, Josefstädterstraße 39, 1080 Vienna, Austria*

(Dated: August 5, 2021)

## SUPPLEMENTAL MATERIALS

### Supplemental Figures

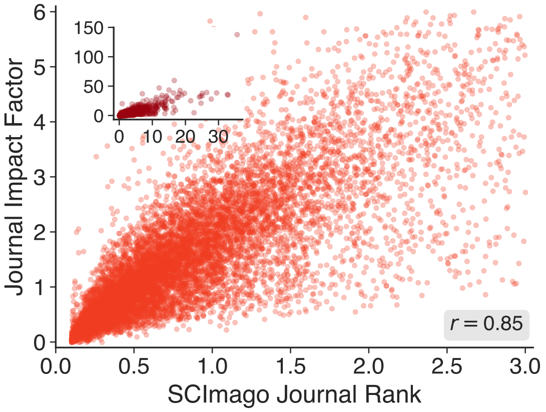


FIG. S1. **Journal Impact Factor (JIF) and SCImago Journal Rank (SJR) are correlated.** Scatter plot of the SJR versus JIF for 11,055 journals present in both data sets for the year 2015. The inset displays the scatter plot considering the full range for which data is available. The Pearson correlation coefficient between these variables is $r = 0.85$, indicating a significant correlation between these journal prestige measures. Results are similar for the other years of our data sets.

* hvr@dfi.uem.br

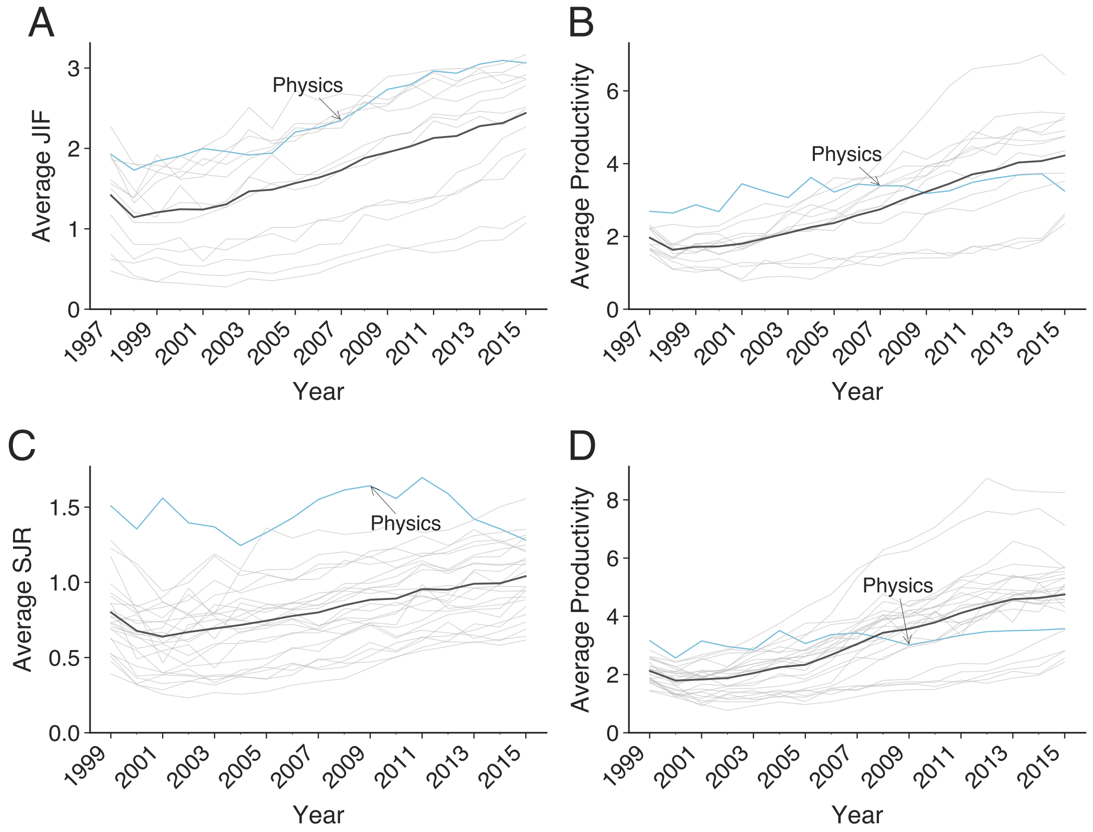


FIG. S2. **Time evolution of the average journal prestige and productivity.** The different gray curves show the time evolution of the (A) average journal prestige and (B) average productivity for the Journal Impact Factor (JIF) data set for all disciplines in our study. Panels (C) and (D) show the same information for the SCImago Journal Rank (SJR) data set. Black curves represent the aggregate behavior for all disciplines, and blue curves illustrate the behavior for Physics. The average values were estimated by using the Huber location estimator (see main text for details).

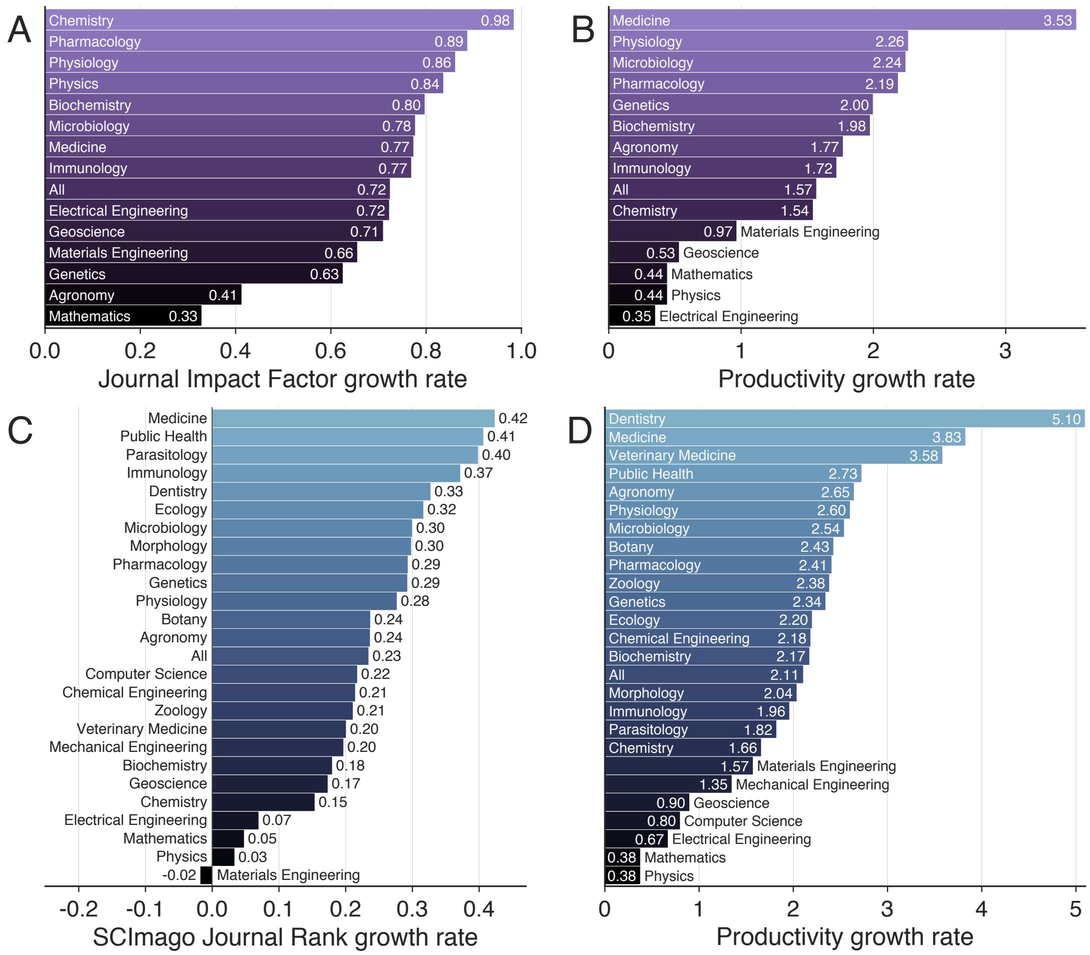


FIG. S3. **Growth rates per decade of journal prestige and productivity.** Panels (A) and (B) show the growth rates per decade of the average journal prestige and productivity estimated from the Journal Impact Factor (JIF) data set. Panels (C) and (D) represent the same for the SCImago Journal Rank (SJR) data set. We estimate these growth rates by fitting a linear model to the time evolution reported in Fig. S2 for every discipline of each data set and when aggregating the behavior of all disciplines (indicated by "all" in these bar plots).

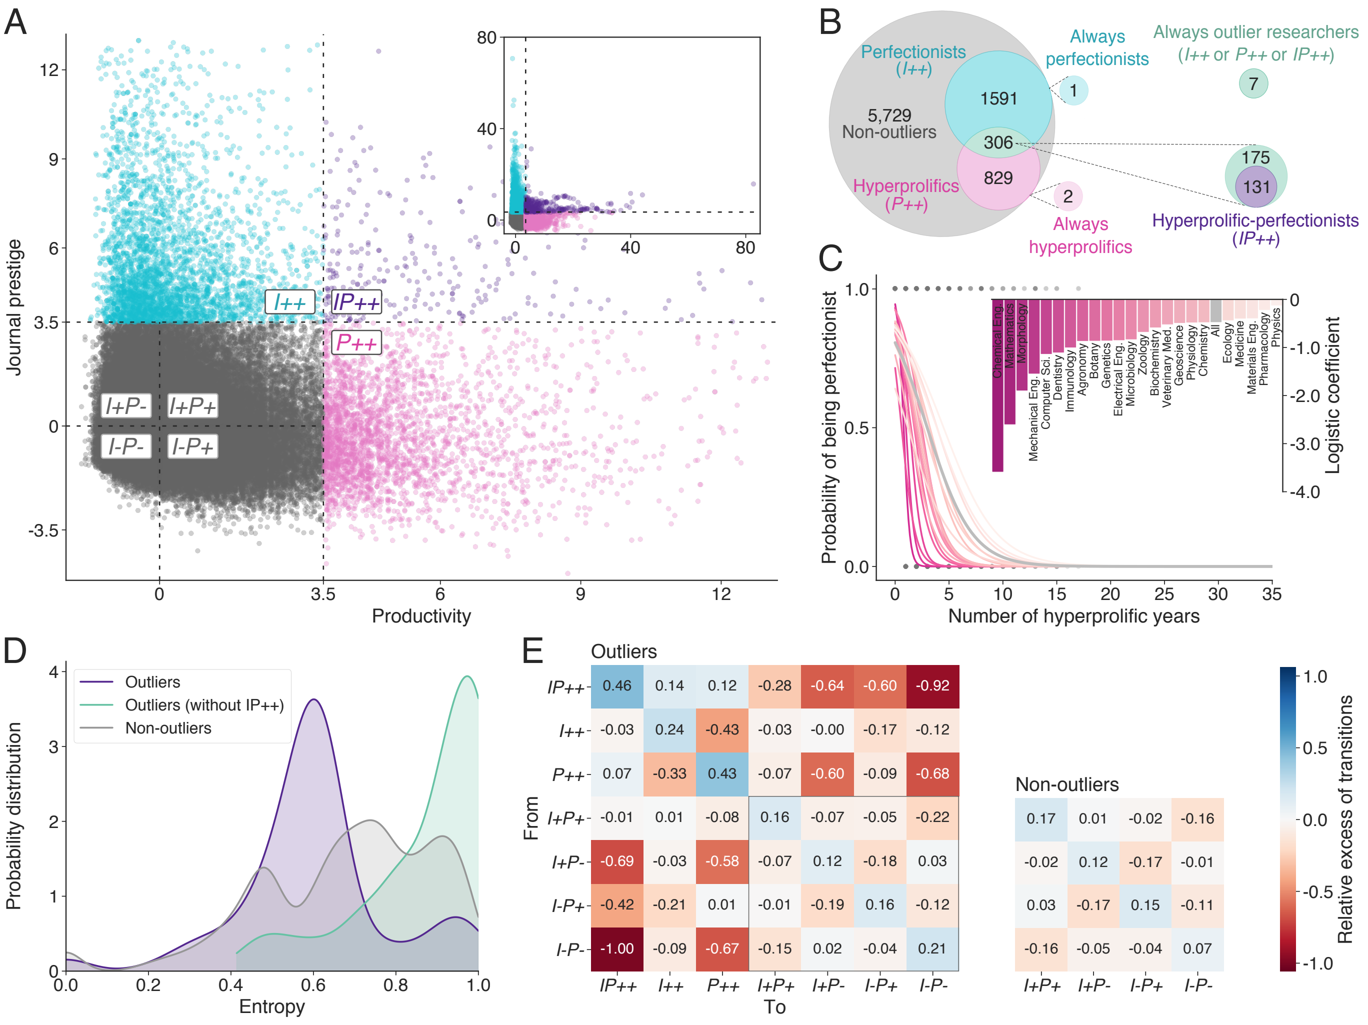


FIG. S4. **Journal prestige versus productivity when considering the SJR data set.** (A) Relation between average journal impact and productivity in standard score units (the inset shows the full range of the plane). Data points represent career years of researchers from the 25 disciplines in the SJR data set. This plane is divided into seven sectors. Three sectors represent career years with overly high performance in journal prestige ($I$++), productivity ($P$++), or both quantities ($IP$++). Four non-outlier sectors represent career years with productivity and journal prestige above ($I$+$P$+) or below ($I$−$P$−) the average, journal prestige below and productivity above the average ($I$−$P$+), and journal prestige above and productivity below the average ($I$+$P$−). (B) Venn diagram showing the set relations among the four categories of researchers. Non-outliers are those with all career years in non-outlier sectors. Perfectionists and hyperprolifics are researchers with at least one career year in sectors $I$++ and $P$++, respectively. Hyperprolific-perfectionists are those having at least one career year within sector $IP$++. (C) Probability of being a perfectionist researcher while having a given number of career years in the hyperprolific sector ($P$++), as estimated via logistic regression (the inset shows the logistic coefficients). The colored curves (and bars) refer to different disciplines, while the gray colored curve represents the aggregate result of all disciplines. Parasitology and Public Health (omitted in this panel) do not display a significant association. (D) Probability distribution of the normalized entropy values associated with the occupation of the plane sectors over researchers' careers. The purple curve shows the results for the occupation of only outlier sectors by outlier researchers and the green curve is the same but after ignoring sector $IP$++. The gray curve shows the entropy distribution for non-outlier researchers. (E) Transition matrix among the plane sectors for outlier (left) and non-outlier (right) researchers. Each cell represents the relative excess of transitions between two sectors compared with a null model corresponding to shuffled versions of researchers' careers for 10,000 realizations.

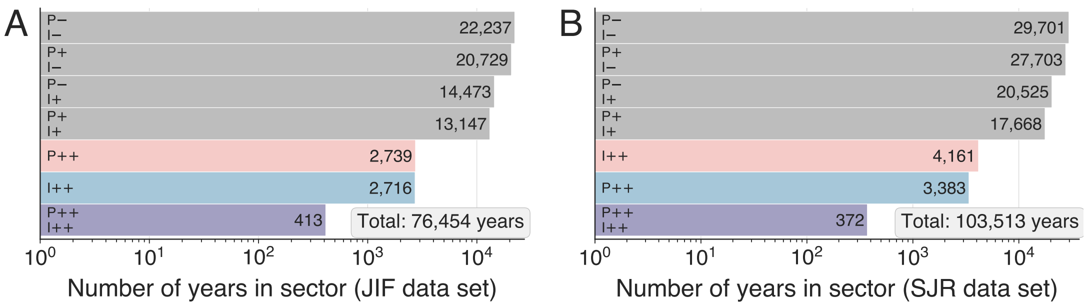


FIG. S5. **Demography of the journal prestige versus productivity plane.** Bar plots display the number of career years in each sector of the journal prestige versus productivity plane. Panel (A) refers to the JIF data set and panel (B) refers to the SJR data set. We note that non-outlier sectors are more populated than outlier sectors. In addition, the $I$–$P$− sector is the most populated sector for both data sets, whereas the $IP$++ sector is the most underpopulated.

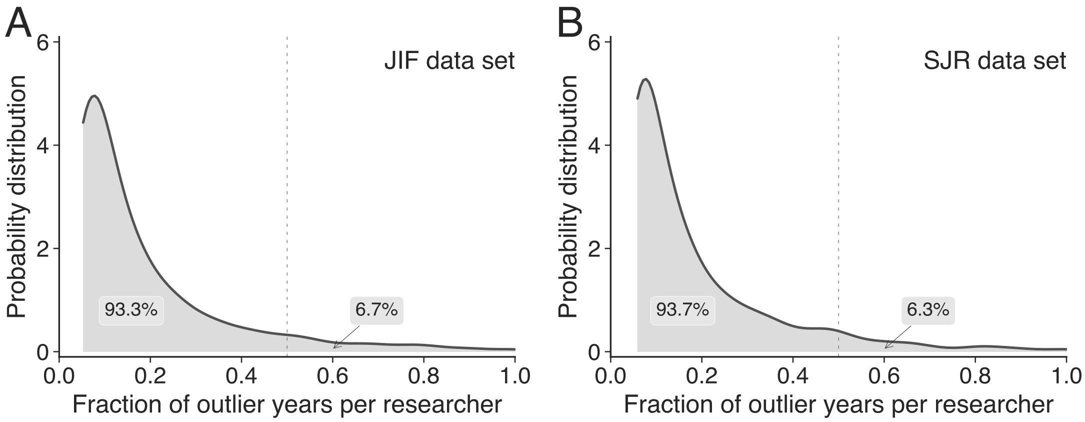


FIG. S6. **Outlier years in scientific careers.** Probability distributions of the fraction of outlier years over the researchers' careers for the (A) JIF data set and the (B) SJR data set. We find that only 6.7% of the outlier researchers have more than 50% of their career years within outlier sectors in the JIF data set. For the SJR data set, only 6.3% of the outlier researchers have more than 50% of their career years within outlier sectors. We further verify that more than 47.6% of researchers are outliers only in one year for the JIF data set and 48.8% of researchers for the SJR data set. Thus, outlier years are quite rare in scientific careers even for outlier scholars.

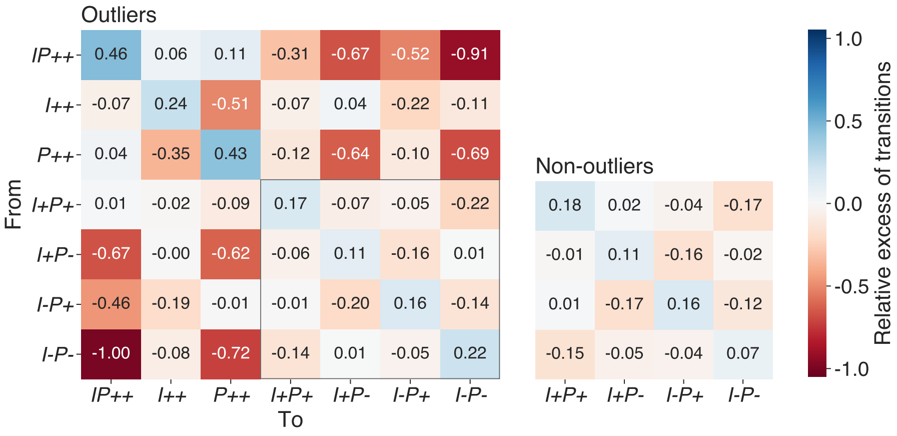


FIG. S7. **Transition matrix among the plane sectors for the SJR data set when considering only the set of disciplines present in the JIF data set.** Each cell represents the relative excess of transitions between two sectors compared with a null model corresponding to shuffled versions of researchers' careers for 10,000 realizations. We note that the transition patterns shown here are very similar to those reported in Fig. S4E.

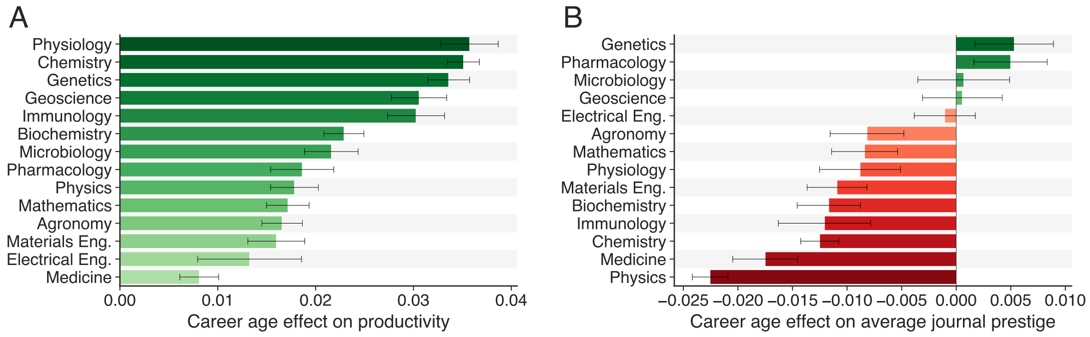


FIG. S8. **Career age effect on productivity and average journal prestige for different disciplines.** Bar plots display the effect of career age on (A) productivity and (B) average journal prestige for each discipline in the JIF data set. We estimate these values by fitting a linear model to the average association between career age and productivity and the average relation between career age average journal prestige (Fig. 2 of the main text) for each discipline. Error bars stand for standard error of the linear coefficients. We observe an increasing trend of productivity with career progression for all disciplines and a downward trend in average journal prestige over career years for most disciplines.

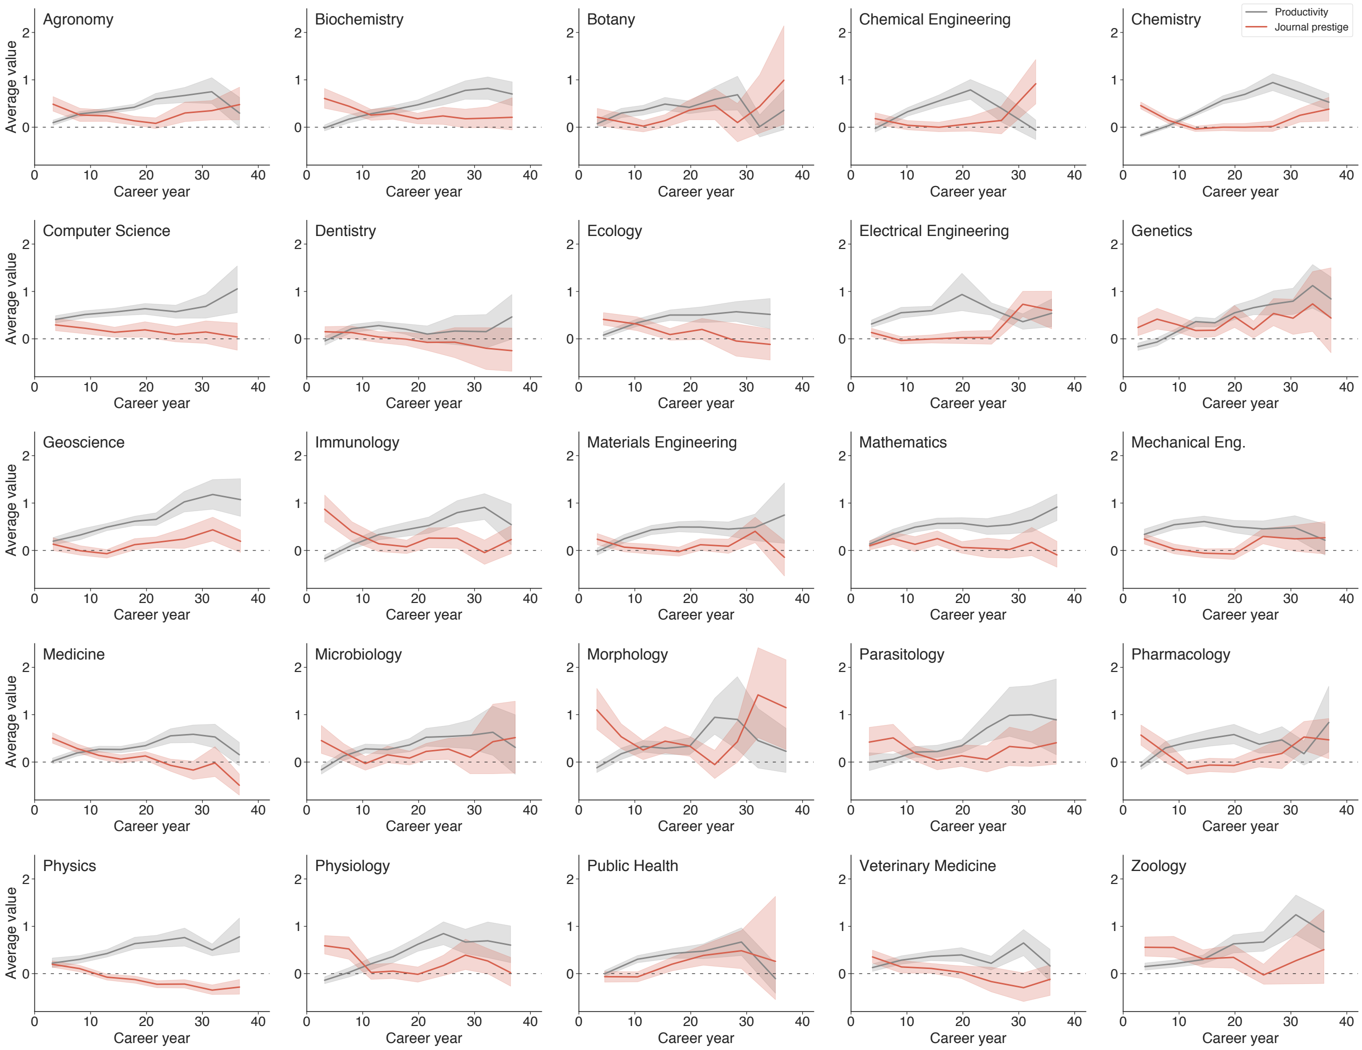


FIG. S9. **Average productivity and journal impact over researchers' careers for different disciplines when considering the SJR data set.** These visualizations show the average productivity (gray curves) and the average journal prestige (red curves) calculated within 5-year sliding windows over career years for each discipline in the SJR data set. Shaded areas correspond to bootstrapping 95% confidence intervals. Average productivity increases with career progression for all disciplines (Fig. S10A) and shows a plateau or small decrease in later career stages for most disciplines. Although some disciplines display more complex patterns, average journal prestige has a subtle downward trend and is usually larger in initial career stages for most disciplines (Fig. S10B).

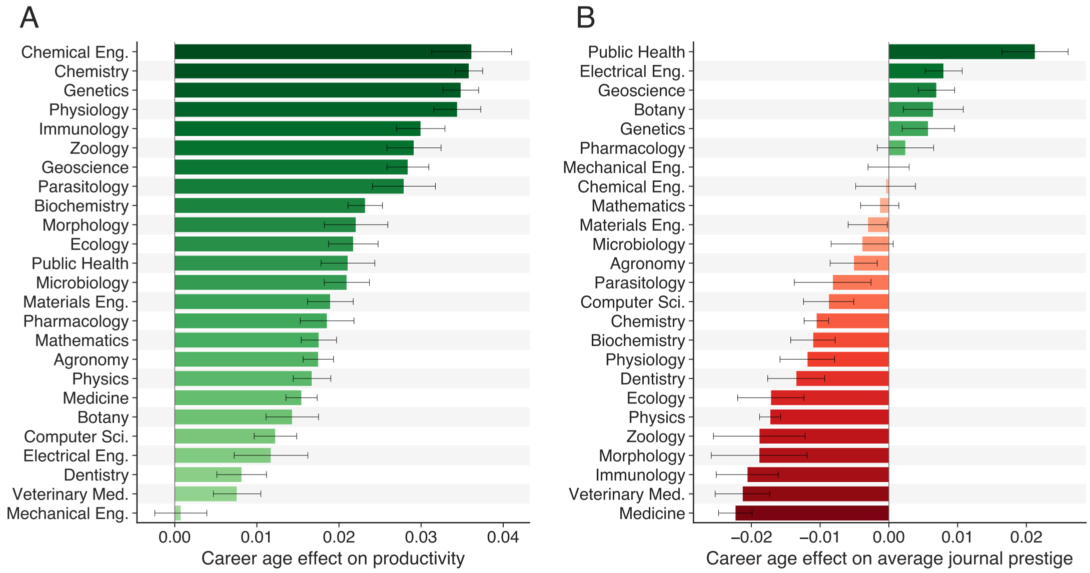


FIG. S10. **Career age effect on productivity and average journal prestige for different disciplines when considering the SJR data set.** Bar plots display the effect of career age on (A) productivity and (B) average journal prestige for each discipline in the SJR data set. We estimate these values by fitting a linear model to the average association between career age and productivity and the average relation between career age average journal prestige (Fig. S9) for each discipline. Error bars stand for standard error of the linear coefficients. We observe an increasing trend of productivity with career progression for all disciplines and a downward trend in average journal prestige over career years for most disciplines.

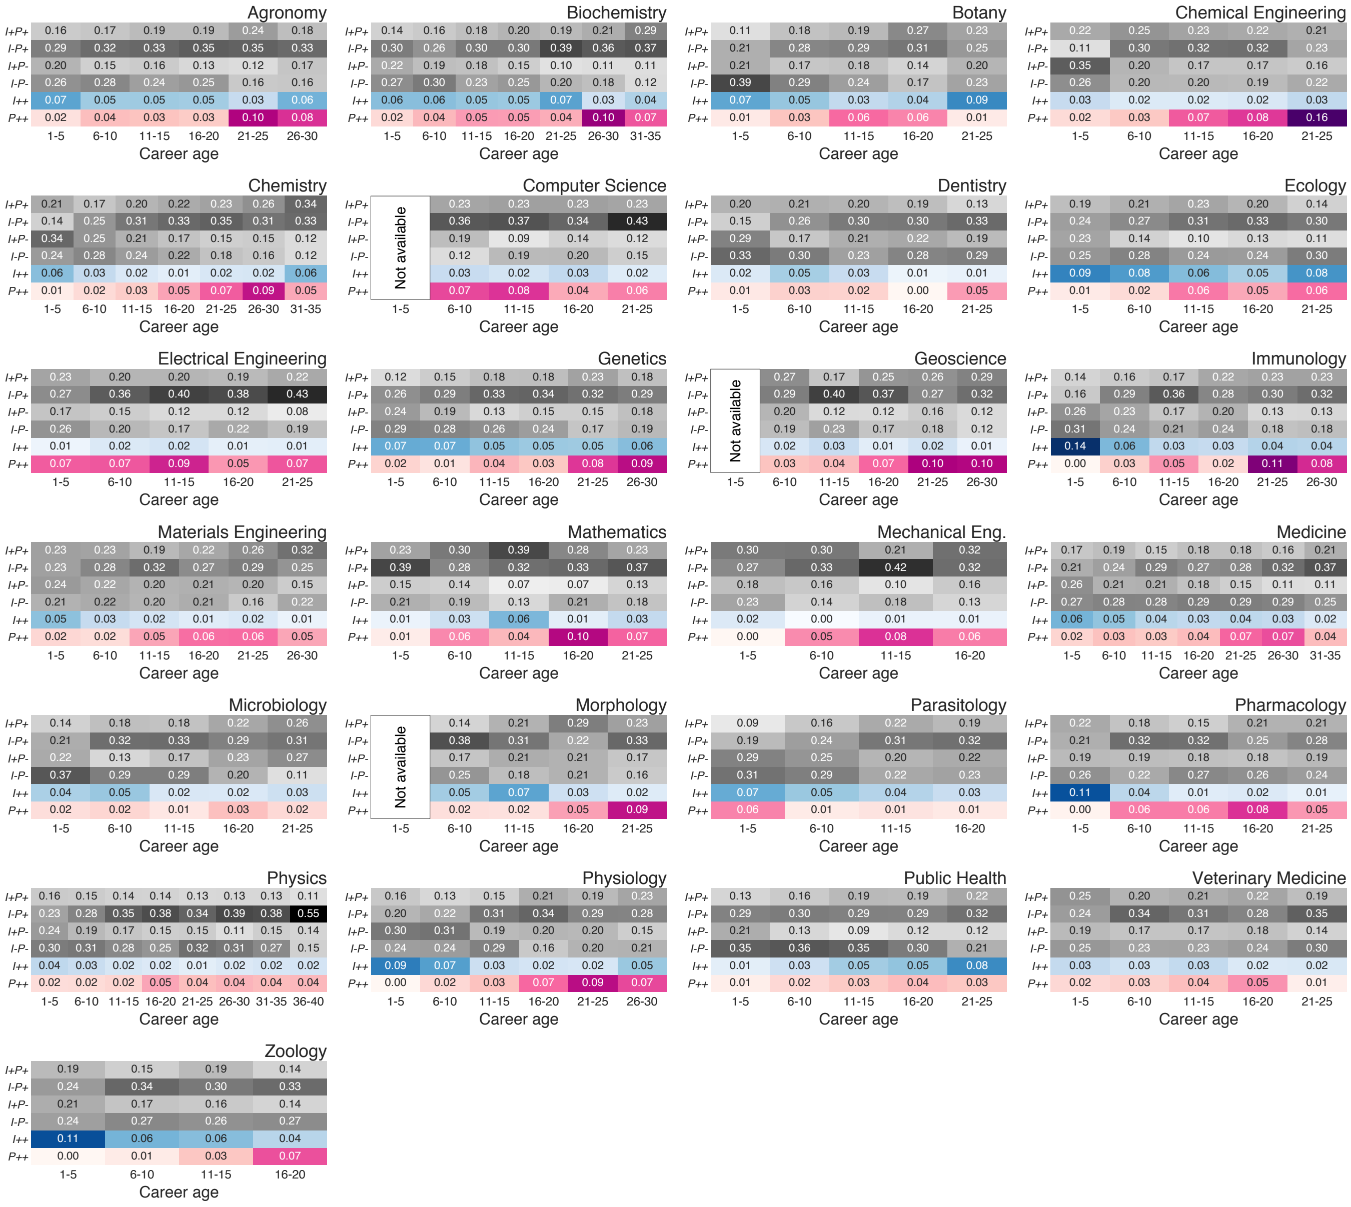


FIG. S11. **Occupation trends in the journal prestige versus productivity plane over researchers' careerss when considering the SJR data set.** These visualizations show the fraction of career years in each non-outlier sector and in outlier sectors $I$++ and $P$++ as a function of researchers' career age for the 25 disciplines in the SJR data set. Columns indicate 5-year intervals and lines represent the different sectors. The same color code indicates the fractions for the non-outlier sectors (gray shades), and the other two color codes are used for the outlier sectors $I$++ (blue shades) and $P$++ (pink shades). Sector $IP$++ is omitted because career years in this sector are very rare. We observe that low-productivity sectors are more populated during initial career years and a shifting trend towards high-productivity sectors in later career stages for most disciplines. Only 5-year intervals having at least 20 researchers are shown in these visualizations.

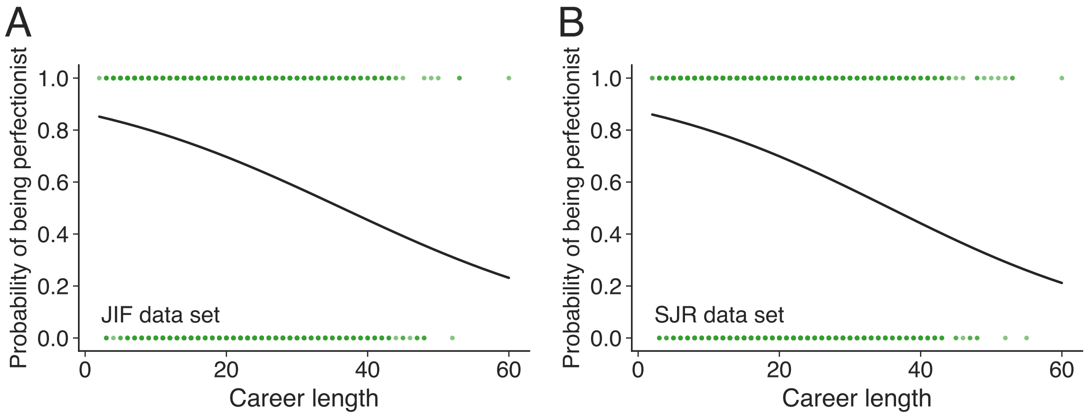


FIG. S12. **Effect of career length on the probability of being a perfectionist.** We estimate the probability of being a perfectionist as a function of the researchers' career length via a logistic regression model (see main text for details). Panel (A) shows this probability for the JIF data set, and panel (B) shows the same analysis for the SJR data set. For the JIF data set, the probability of being a perfectionist decreases from 79% to 58% when career length increases from 10 to 30 years. For the SJR data set, this probability decreases from 80% to 58% for the same variation in career length.

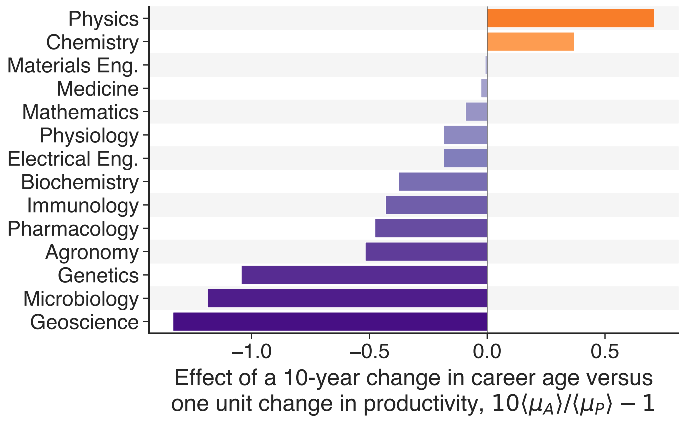


FIG. S13. **Comparison between the effects of career age and productivity on average journal prestige.** Bar plot comparing the effect of a 10-year career progression with the effect of increasing one unit in productivity ($z$-score) for a typical researcher of each discipline in the JIF data set. These values represent the fraction of how larger or smaller is the effect of career age compared with the effect of productivity (that is, $10\langle\mu_A\rangle/\langle\mu_P\rangle - 1$, where $\langle\mu_A\rangle$ and $\langle\mu_P\rangle$ are the average values of $\mu_A$ and $\mu_P$ for each discipline, respectively). Thus, fractions around zero indicate that a 10-year increase in career age affects journal impact similarly to a rise in one unit in productivity. Positive values indicate that a 10-year change in career age affects more journal impact than one unity of productivity, while negative values indicate that productivity has a larger impact on journal impact. For the JIF data set, a 10-year career progression has a larger effect only for Chemistry and Physics.

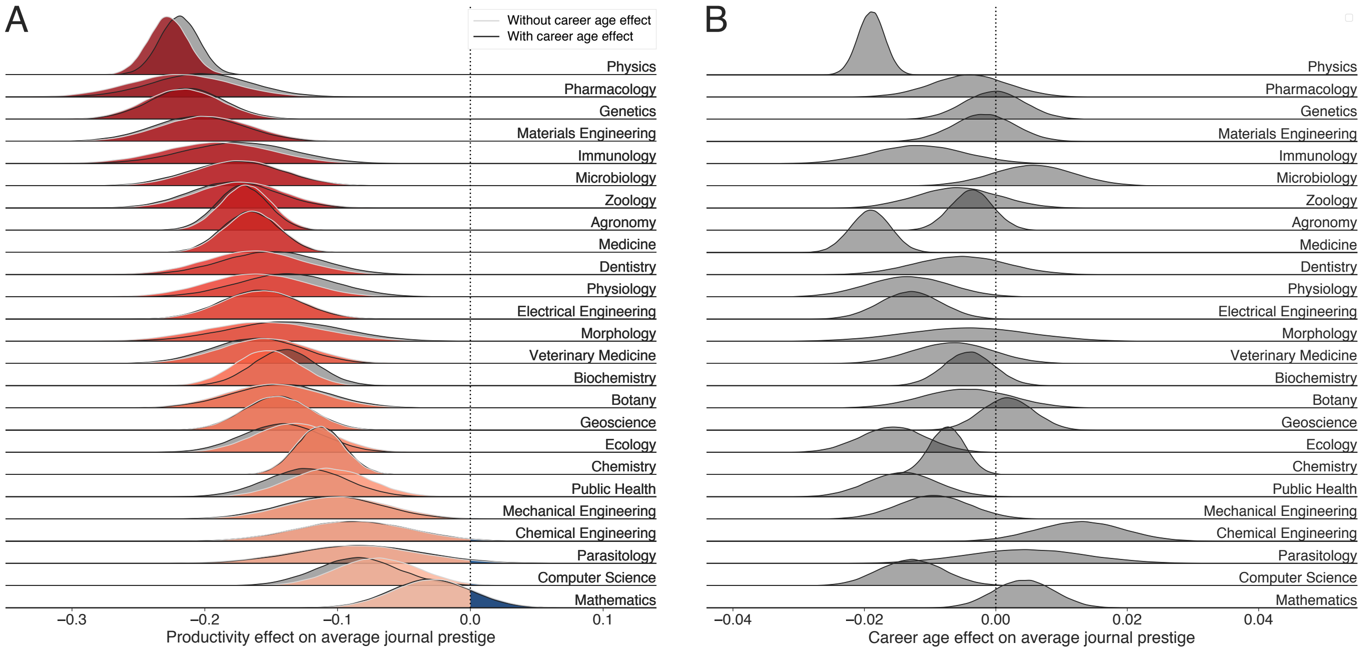


FIG. S14. **Effect of productivity on journal prestige for non-outlier researchers when considering the SJR data set.** (A) Posterior probability distributions of the average value of the linear coefficient ($\mu_P$) when considering the association between productivity and journal impact for non-outlier researchers of each discipline. The colored-filled curves represent the results without accounting for the effects of career age, while the gray-filled curves show the distributions of $\mu_P$ after including career age as a confounding factor in the hierarchical Bayesian model (see Methods for details). (B) Posterior probability distributions of the average value of the linear coefficient ($\mu_A$) related to the effect of career age on journal impact for non-outlier researchers of each discipline.

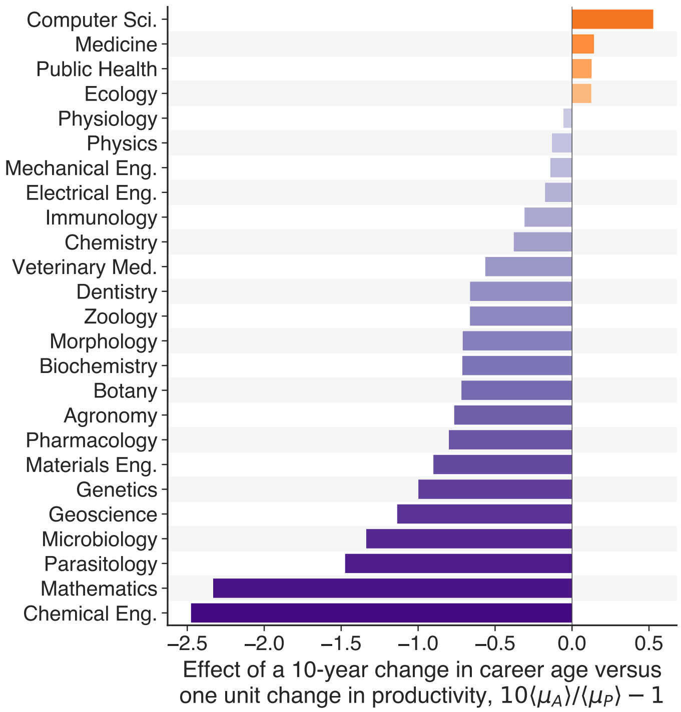


FIG. S15. **Comparison between the effects of career age and productivity on average journal prestige when considering the SJR data set.** Bar plot comparing the effect of a 10-year career progression with the effect of increasing one unit in productivity ($z$-score) for a typical researcher of each discipline in the SJR data set. These values represent the fraction of how larger or smaller is the effect of career age compared with the effect of productivity (that is, $10\langle\mu_A\rangle/\langle\mu_P\rangle - 1$, where $\langle\mu_A\rangle$ and $\langle\mu_P\rangle$ are the average values of $\mu_A$ and $\mu_P$ for each discipline, respectively). Thus, fractions around zero indicate that a 10-year increase in career age affects journal impact similarly to a rise in one unit in productivity. Positive values indicate that a 10-year change in career age affects more journal impact than one unity of productivity, while negative values indicate that productivity has a larger impact on journal impact. For the SJR data set, a 10-year career progression has a larger effect only for Computer Science, Ecology, Medicine and Public Health.

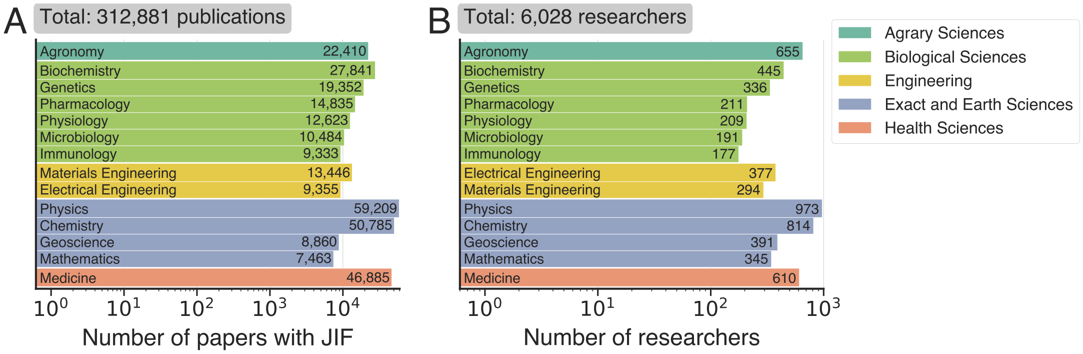


FIG. S16. **Number of publications and researchers in the Journal Impact Factor (JIF) data set.** Panel (A) shows the total number of articles and panel (B) shows the total number of researchers for each discipline in the JIF data set. The bar colors represent the different fields of science covered by our data set.

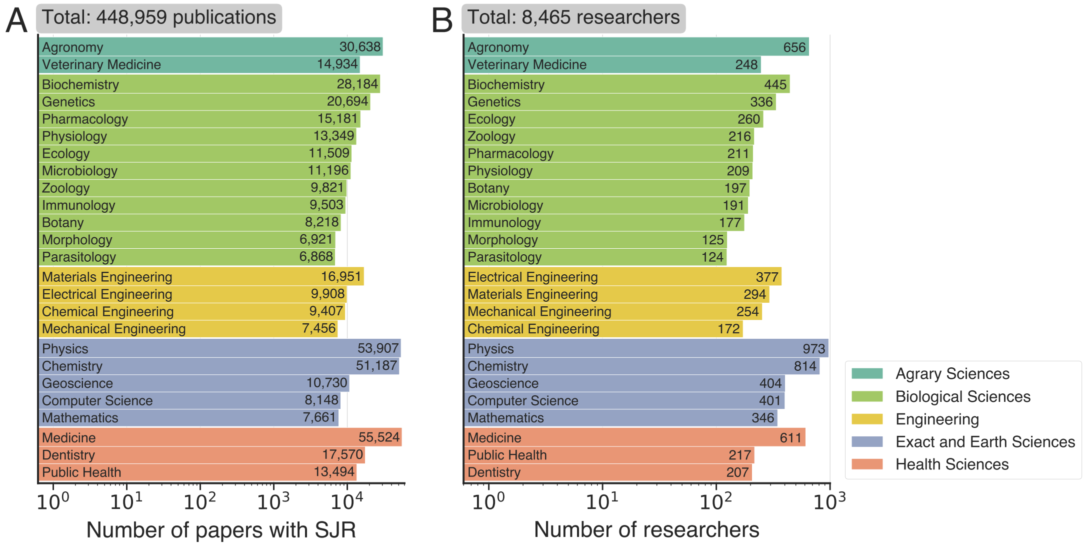


FIG. S17. **Number of publications and researchers in the SCImago Journal Rank (SJR) data set.** Panel (A) shows the total number of articles and panel (B) shows the total number of researchers for each discipline in the SJR data set. The bar colors represent the different fields of science covered by our data set.

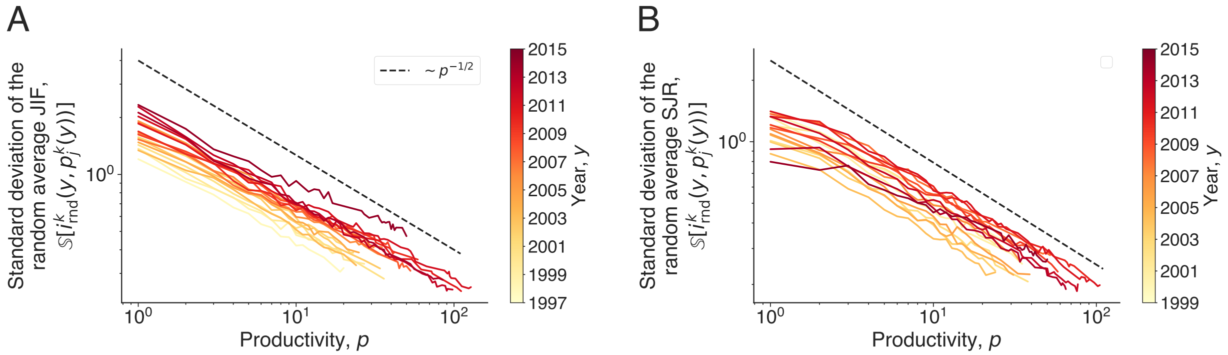


FIG. S18. **Size effect of productivity on volatility of average journal prestige.** (A) Standard deviation ($\mathbb{S}[i^k_{\rm rnd}(y, p^k_j(y))]$) of the average Journal Impact Factor (JIF) estimated from a 1,000 random samples of $p$ publications from researchers of Physics as a function of $p$ for all years available in the JIF data set. The color code refers to each year of the data set and dashed line represents the behavior expected by the Central Limit Theorem. We observe that the standard deviation decreases with $p$, confirming that low productivity is associated with high variability, while high productivity is associated with low variability in average journal prestige. Panel (B) show the same results when considering the SCImago Journal Rank (SJR) as the journal prestige indicator. Similar behavior is observed for all years and disciplines for the JIF and SJR data sets.

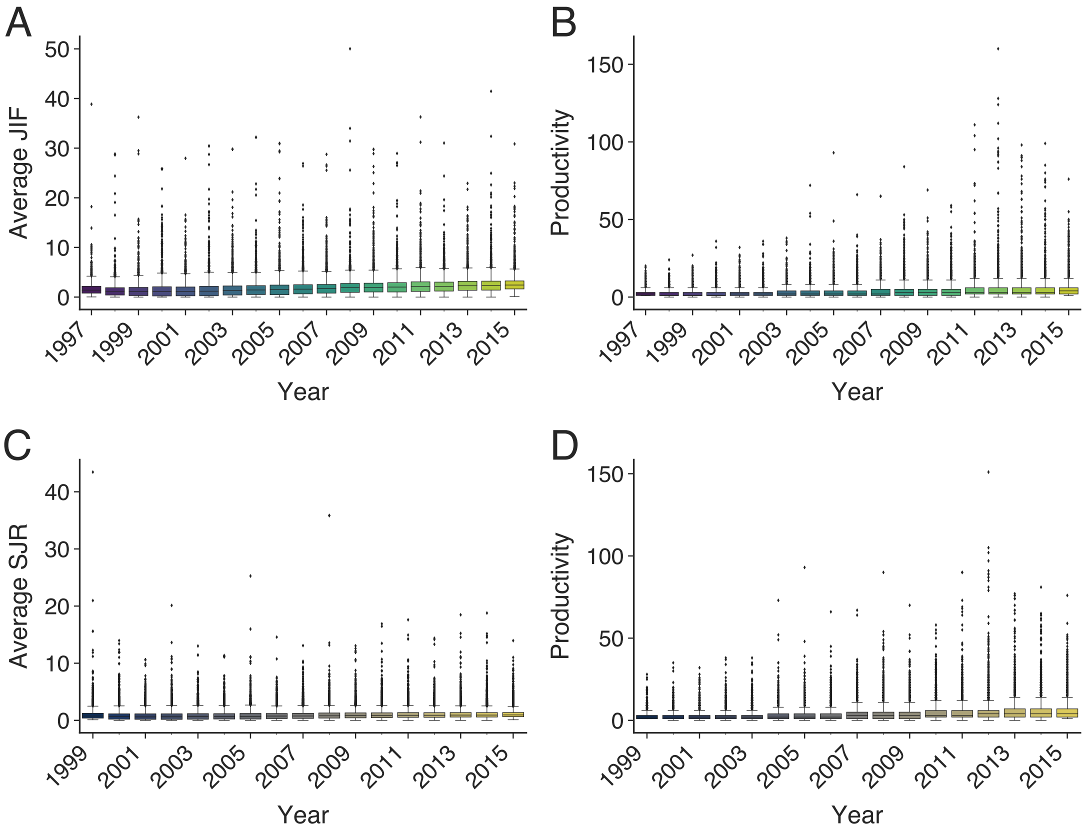


FIG. S19. **Outlier values of average journal prestige and productivity.** Box plots depict the degree of dispersion of the (A) average Journal Impact Factor (JIF) and (B) productivity of researchers in the JIF data set over the years. Panels (C) and (D) show the analagous results for the SCImago Journal Rank (SJR) data set. We observe the presence of extreme observations in all years, which are represented by black markers located beyond whiskers (here defined as 1.5 times the interquartile range).

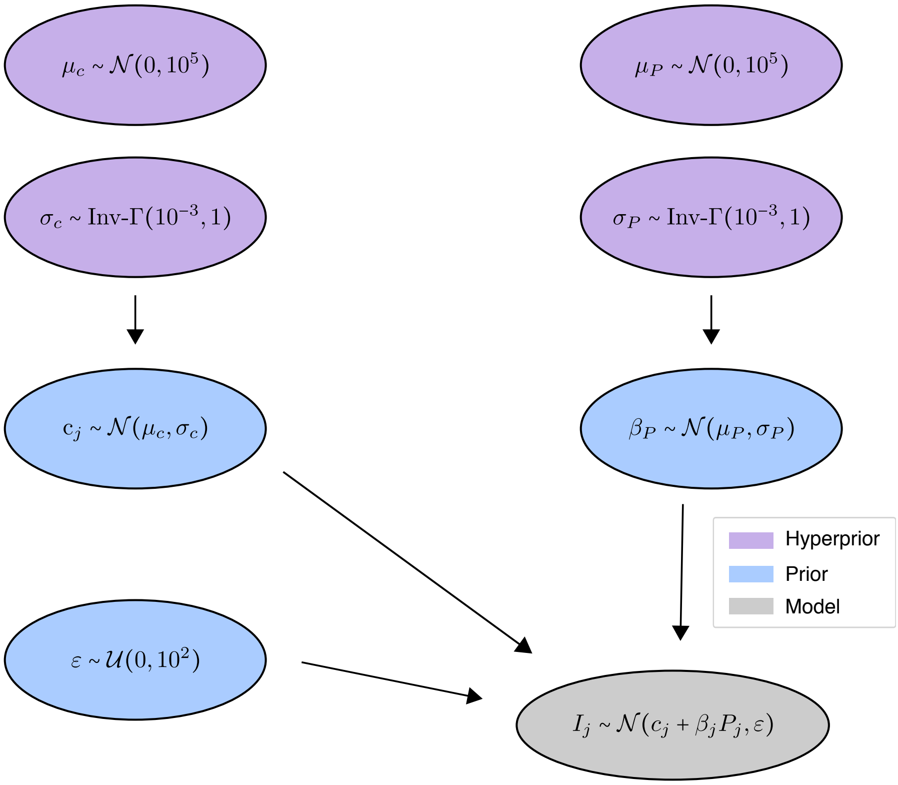


FIG. S20. **Visual representation of the Bayesian hierarchical model defined by Eq. 1.** Schematic description of the Bayesian hierarchical model (Eq. 1) used for estimating the effect of productivity on journal prestige for non-outlier researchers. Purple colored shapes represent hyperprior distributions, blue colored shapes represent prior distributions, and the gray colored shape represents the overall structure of our hierarchical model.

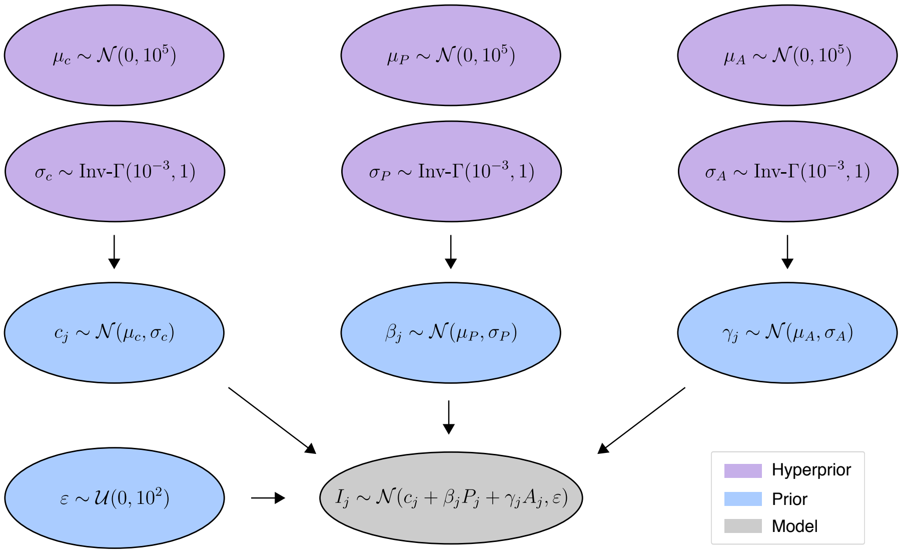


FIG. S21. **Visual representation of the Bayesian hierarchical model with career age independent variable (Eq. 3).** Schematic description of the Bayesian hierarchical model used for estimating the effect of productivity and career age on journal prestige for non-outlier researchers (Eq. 3). Purple colored shapes represent hyperprior distributions, blue colored shapes represent prior distributions, and the gray colored shape represents the overall structure of our hierarchical model.

**Supplemental Tables**

TABLE S1. **Description of the Journal Impact Factor (JIF) data set used in the Bayesian hierarchical analysis.** Number of researchers and data points for each discipline in the JIF data set after filtering out researchers with careers shorter than five years.

| Discipline | Number of researchers | Number of data points |
|---|---|---|
| Agronomy | 462 | 4523 |
| Biochemistry | 258 | 3482 |
| Chemistry | 577 | 7701 |
| Electrical Engineering | 232 | 2302 |
| Genetics | 210 | 2709 |
| Geoscience | 229 | 2195 |
| Immunology | 109 | 1415 |
| Materials Engineering | 210 | 2496 |
| Mathematics | 212 | 2128 |
| Medicine | 357 | 4765 |
| Microbiology | 131 | 1670 |
| Pharmacology | 147 | 2003 |
| Physics | 686 | 9348 |
| Physiology | 136 | 1757 |

TABLE S2. **Description of the SCImago Journal Rank (SJR) data set used in the Bayesian hierarchical analysis.** Number of researchers and data points for each discipline in the SJR data set after filtering out researchers with careers shorter than five years.

| Discipline | Number of researchers | Number of data points |
|---|---|---|
| Agronomy | 408 | 4391 |
| Biochemistry | 239 | 3123 |
| Botany | 124 | 1359 |
| Chemical Engineering | 124 | 1536 |
| Chemistry | 566 | 7314 |
| Computer Science | 230 | 2036 |
| Dentistry | 151 | 1937 |
| Ecology | 160 | 1821 |
| Electrical Engineering | 239 | 2297 |
| Genetics | 188 | 2409 |
| Geoscience | 273 | 2725 |
| Immunology | 102 | 1299 |
| Materials Engineering | 204 | 2535 |
| Mathematics | 215 | 2147 |
| Mechanical Engineering | 187 | 1921 |
| Medicine | 361 | 4983 |
| Microbiology | 131 | 1698 |
| Morphology | 71 | 956 |
| Parasitology | 72 | 956 |
| Pharmacology | 142 | 1878 |
| Physics | 670 | 8474 |
| Physiology | 133 | 1672 |
| Public Health | 144 | 1734 |
| Veterinary Medicine | 178 | 2138 |
| Zoology | 126 | 1418 |
